# Supplementary material for: How to unloop a self-adherent sheet
Source: arXiv:2009.07323 ancillary file (2021-04-20)
Supplement: Supplementary file 1 [file SupplementaryInformation.pdf]

# Supplementary Information:
# How to unloop a self-adherent sheet

Twan J.S. Wilting, Martin H. Essink, Hanneke Gelderblom, and Jacco H. Snoeijer

March 5, 2021

## 1 Experimental details

In the main text we primarily focus on peeling characteristics of tape A, except for the inset of Fig. 4. Here we show the robustness of the results for the other tapes, as listed in Table 1 of the main paper. Figure S.1a shows evolution of the peeling curvature for the four tapes. In all cases the curvature increases as the loop shrinks in size, and for $a/\ell_{ea} \gtrsim 3$, we find a good match between the model of equation (5). The behavior at smaller loop sizes is not universal, as explained in the text. However, the loop rupture always occurs very close to the point where $\kappa_b = \kappa_a$, for all tapes.

In Fig. S.1b we have a closer look at the results for tape D, which consists of two layers of tape A to show the influence of tape thickness $t$. The elasto-adhesive length $\ell_{ea}$ as determined from the measurements with tape D is approximately double that of tape A. This is slightly less than the ratio of $2\sqrt{2}$ predicted by the typical thickness dependence of an elastica $B \sim t^3$, which can be attributed to the soft adhesive layer between the two tapes. We see that the peeling curvature is in line with expectations, as well as the prediction for the point of rupture. The inset of this figure shows the collapse of the critical loop size $a_c$ measurements onto the power law predicted in equation (9) of the main paper.

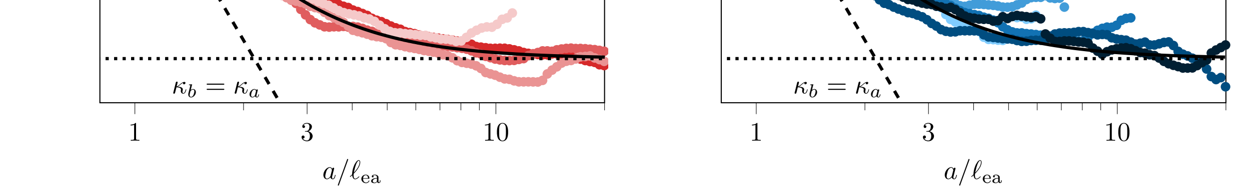


Figure S.1: Plot of the dimensionless peeling curvature $\kappa_b \ell_{ea}$ versus loop size $a/\ell_{ea}$ averaged over multiple measurements. The solid line is the simplified model, equation (5) in the main text, the dotted horizontal line shows $\kappa_{iso} = \sqrt{2}/\ell_{ea}$. **(a)** For all the four tapes listed in Table 1, at a peeling velocity $v = 4.2 \cdot 10^{-2}$ mm/s. **(b)** For tape D at various peeling velocities ranging between $v = 4.2 \cdot 10^{-3}$ mm/s and $v = 1.2$ mm/s. The symbols "+" indicate the model prediction for rupture with $\alpha = 4.3$. Inset: Relation between $a_c$ and $\ell_{ea}^{2/3} t^{1/3}$, for both a single and a double layer of tape. The solid line represents the asymptotic result predicted by the model given by (S.12), with $\alpha = 4.3$.

# 2 Modeling details

## 2.1 Energy release rate

In the main paper we provide the expression for the total mechanical energy of the elastica (1), as

$$\mathcal{E}_B - \mathcal{W} = \int_0^L ds \left(\frac{1}{2}B\theta'^2 - f\sin(\theta)\right). \tag{S.1}$$

However, this expression does not yet include the constraints that define the contact points $s = a$ and $s = b$; these constraints are important to compute the energy released during peeling. The contact points are defined by the condition that the loop is closed. In Cartesian coordinates, with $y$ taken as the normal distance with respect to the symmetry axis, this condition implies $y(a) = y(0) = 0$, while similarly $y(b) = 0$. The former constraint can be enforced by adding $(f_a \int_0^a ds\ \sin\theta)$ to the right-hand side of (S.1), where $f_a$ is the internal force in the loop. The constraint on $y(b)$ is already accounted for in (S.1) by the expression for the work done by the peeling force. From now on we write $f = f_b$. Finally, one needs to impose $\theta(a) = \theta(b) = 0$, ensuring that $\theta$ remains continuous on the entire domain. These constraints are imposed by Lagrange-multiplier terms $\lambda_a\theta(a)$ and $\lambda_b\theta(b)$, added to the mechanical energy. Finally, noting that $\theta = 0$ for $a < s < b$, the functional to be minimized reads:

$$\begin{aligned}\mathcal{E}_B - \mathcal{W} &= \int_0^a ds\ \left(\frac{1}{2}B\theta'^2 - f_a\sin(\theta)\right) + \lambda_a\theta(a)\\ &\quad + \int_b^L ds\ \left(\frac{1}{2}B\theta'^2 - f_b\sin(\theta)\right) + \lambda_b\theta(b).\end{aligned} \tag{S.2}$$

By introducing the Lagrangians $\mathcal{L}_a$ and $\mathcal{L}_b$ for each side of the contact this expression simplifies to

$$\mathcal{E}_B - \mathcal{W} = \int_0^a ds\ \mathcal{L}_a(\theta',\theta) + \lambda_a\theta(a) + \int_b^L ds\ \mathcal{L}_b(\theta',\theta) + \lambda_b\theta(b). \tag{S.3}$$

The variation of the total mechanical energy $\delta(\mathcal{E}_B - \mathcal{W})$ with respect to $\theta(s)$ gives

$$\begin{aligned}&\delta(\mathcal{E}_B - \mathcal{W}) = 0 =\\ &- \frac{\partial\mathcal{L}_a}{\partial\theta'}\delta\theta\bigg|_{s=0} + \left(\lambda_a + \frac{\partial\mathcal{L}_a}{\partial\theta'}\right)\delta\theta\bigg|_{s=a} + \int_0^a ds\,\delta\theta\left(\frac{\partial\mathcal{L}_a}{\partial\theta} - \frac{\mathrm{d}}{\mathrm{d}s}\frac{\partial\mathcal{L}_a}{\partial\theta'}\right)\\ &+ \left(\lambda_b - \frac{\partial\mathcal{L}_b}{\partial\theta'}\right)\delta\theta\bigg|_{s=b} + \frac{\partial\mathcal{L}_b}{\partial\theta'}\delta\theta\bigg|_{s=L} + \int_b^L ds\,\delta\theta\left(\frac{\partial\mathcal{L}_b}{\partial\theta} - \frac{\mathrm{d}}{\mathrm{d}s}\frac{\partial\mathcal{L}_b}{\partial\theta'}\right).\end{aligned} \tag{S.4}$$

Hence, for the loop region ($0 \le s \le a$) and the peeling region ($b \le s \le L$) one obtains the elastica equations

$$\frac{\partial\mathcal{L}_{a,b}}{\partial\theta} - \frac{\mathrm{d}}{\mathrm{d}s}\frac{\partial\mathcal{L}_{a,b}}{\partial\theta'} = B\theta'' + f_{a,b}\cos\theta = 0, \tag{S.5}$$

given as (2) in the main text. The boundary terms $\delta\theta(0) = \delta\theta(L) = 0$ vanish naturally, but at $s = a$ and $s = b$ we determine the Lagrange multipliers as

$$\lambda_a = -\frac{\partial\mathcal{L}_a}{\partial\theta'}\bigg|_{s=a}, \qquad \lambda_b = \frac{\partial\mathcal{L}_b}{\partial\theta'}\bigg|_{s=b}. \tag{S.6}$$

To find the energy release rates at $s = a$ and $s = b$ upon propagation of the contact zone, we calculate the variation of the mechanical energy with the location of the contact lines. Using again that $\theta(a) = \theta(b) = 0$,

we find the energy release rates

$$\frac{\partial\left(\mathcal{E}_B-\mathcal{W}\right)}{\partial a} = \left.\left(\ \ \mathcal{L}_a+\lambda_a\theta'\right)\right|_{s=a} = -\frac{1}{2}B\theta'(a)^2, \tag{S.7}$$

$$\frac{\partial\left(\mathcal{E}_B-\mathcal{W}\right)}{\partial b} = \left.\left(-\mathcal{L}_b+\lambda_b\theta'\right)\right|_{s=b} = \ \ \frac{1}{2}B\theta'(b)^2, \tag{S.8}$$

which are given as Eqs. (3) and (4) in the main text.

## 2.2 Asymptotic solution at rupture

To find the scaling of the critical loop size, we solve (6,7), with interaction energy $\mathcal{E}_{\text{int}}$ given by (8). The interaction energy involves $\kappa_b$ and $\kappa_a$. The confinement of the loop gives that $\kappa_a = 3.028/a$, so that the its derivative gives a contribution to $\partial\mathcal{E}_{\text{int}}/\partial a$ in (7). By contrast, $\kappa_b$ is not constrained geometrically, so it remains constant during the differentiation. With this, one can solve (6,7) in terms of the peeling curvature $\kappa_b$ and the length of the contact zone $w$, which gives

$$\kappa_b = \sqrt{\frac{2}{\ell_{\text{ea}}^2}+\kappa_a^2\left(1+4\frac{\alpha^2t^2}{a^2}-2\sqrt{2}\frac{\alpha t}{a}\sqrt{2\frac{\alpha^2t^2}{a^2}+1}\right)}, \tag{S.9}$$

$$w = \frac{2\alpha^2t^2\left(\kappa_b-\kappa_a\right)}{3.028}\left(1+\sqrt{\frac{1}{2}\frac{a^2}{\alpha^2t^2}+1}\right). \tag{S.10}$$

Rupture appears when $w = 0$, so that the critical loop size $a_c$ corresponds to $\kappa_b = \kappa_a = 3.028/a$. In this case, assuming $t \ll \ell_{\text{ea}}$, (S.9) reduces to

$$\frac{2}{\ell_{\text{ea}}^2}\frac{a_c^2}{3.028^2} = 2\sqrt{2}\alpha\frac{\ell_{\text{ea}}}{a_c}\left(\frac{t}{\ell_{\text{ea}}}\right)+\mathcal{O}\left(\frac{t}{\ell_{\text{ea}}}\right)^2, \tag{S.11}$$

from which we obtain the asymptotic result which is presented as (9),

$$a_c = \left(2\times 3.028^4\right)^{1/6}\left(\alpha t\ell_{\text{ea}}^2\right)^{1/3}. \tag{S.12}$$

Similarly, expanding (S.10) around $a = a_c$, assuming $t \ll \ell_{\text{ea}}$ yields the asymptotic scaling of $w$ with $a$ near the point of rupture, presented as (10)

$$w = \left(\frac{108}{3.028^4}\right)^{1/3}\left(\frac{\alpha t}{\ell_{ea}}\right)^{4/3}\left(a-a_c\right). \tag{S.13}$$

# 3 Movies

Movie S.1: Recording of the unlooping of tape A that corresponds to the time-series and results of Figs. 1 and 2 in the main text.

Movie S.2: Close-up recording of the contact zone of tape A during peeling, as shown in the snapshots in Fig. 5.

Movie S.3: Typical recording for the peeling of a lengthy contact zone of approximately 1.5 cm for tape A. The tape starts to unloop when the contact zone is reduced to about $300-400\,\mu$m.

Movie S.4: Recording of the unlooping of a plastic sheet (thickness 0.125 mm) held together by a lubricant (petrolatum). When the length of the contact $w \approx 5$ mm the contact starts to propagate and the loop shrinks in size. Note that the petrolatum accumulates at the peeling side leaving clumps behind.

Movie S.5: Recording or the rolling motion and contact zone propagation of an adhesive tape over a surface.
